# Supplementary material for: LEVA: Using Large Language Models to Enhance Visual Analytics
Source: arXiv:2403.05816 source file (2024-03-09)
Supplement: Supplementary file 1 [file appendix-develop.tex]

\subsection{Integrate a VA system with LEVA}
\label{appendix:develop}
